# Supplementary material for: Archives of Photographic PLates for Astronomical USE (APPLAUSE) Digitisation of astronomical plates and their integration into the International Virtual Observatory
Source: arXiv:2404.17355 source file (2024-04-26)
Supplement: Supplementary file 1 [file appendix.tex]

\onecolumn
\section{Supplemental tables}

\begin{table*}[h]
\centering
\begin{tabular}{ c  l  l  c r  r  r  r }
\hline\hline
Archive\_id&Archive\_name (Instrument) & Institute & Period& Plates & Scans & processed & not processed\\
\hline
001 & Zeiss Triplet (P) & AIP & 1909--1938 & 4921 & 4915 & 2097 & 2818\\
%\hline
002 & Carte du Ciel  (P)  & AIP & 1893--1924 & 979 & 953 & 0 & 953 \\
%\hline
003 & Great Schmidt Camera  (P)  & AIP & 1952--1970 & 508 & 508 & 413 & 95\\
%\hline
004 & Small Schmidt Camera  (P) & AIP & 1949--1967 & 113 & 101 & 14 & 87\\
%\hline
005 & Ross Camera  (P)  & AIP & 1956--1956 & 64 & 62 & 59 & 3\\
%\hline
006 & Einstein Turm Solar Plates  (P) & AIP & 1943--1991 & 3613 & 3613 & 3613 & 0\\
%\hline
101 & Lippert-Astrograph (HH) & HS & 1912--1972 & 8750 & 13\,764 & 11\,289 & 414\\
%\hline
102 & Grosser Schmidt-Spiegel (HH) & HS & 1954--1975 & 5323 & 7463 & 5146 & 215\\
%\hline
103 & 1m-Spiegelteleskop (HH) & HS & 1911--1972 & 7643 & 7538 & 5409 & 108\\
%\hline
104 & HSS (Calar Alto) & HS & 1980--1998 & 3255 & 4388 & 2644 & 23\\
%\hline
105 & AG-Teleskop (Bonn) &HS & 1926--1958 & 754 & 1454 & 1309 & 145\\
%\hline
106 & AG-Teleskop (HH) &HS & 1927--1973 & 3529 & 7019 & 6848 & 171\\
%\hline
107 & Doppel-Reflektor (HH) & HS & 1934--1957 & 1642 & 2055 & 1897 & 157\\
%\hline
108 & ESO telescopes (La Silla) & HS & 1974--1998 & 2099 & 2713 & 918 & 484\\
%\hline
109 & Grosser Refraktor (HH) & HS & 1914--1985 & 2602 & 2757 & 938 & 1780\\
%\hline
110 & Kleiner Schmidt-Spiegel II (HH) & HS & 1952--1979 & 1566 & 1152 & 852 & 161\\
%\hline
111 & Schmidtsches Spiegelteleskop (HH) & HS & 1931--1968 & 1746 & 1985 & 933 & 421\\
%\hline
202 & Metcalf Telescope (South Africa) & DKRSB & 1963--1972 & 2718 & 2705 & 2701 & 4\\
%\hline
203 & BSSP (South Africa) & DKRSB & 1963--1970 & 12\,565 & 12\,513 & 12\,503 & 9\\
%\hline
204 & BSSP (New Zealand) & DKRSB & 1967--1976 & 5266 & 5243 & 5242 & 1\\
%\hline
205 & BSSP (Argentina) & DKRSB & 1969--1972 & 870 & 824 & 823 & 1\\
%\hline
206 & Zeiss Objective (South Africa) & DKRSB & 1964--1970 & 694 & 690 & 676 & 14\\
%\hline
207 & Ross B Camera (South Africa) & DKRSB & 1964--1966 & 698 & 696 & 694 & 2\\
%\hline
208 & BNSP Astrograph & DKRSB & 1912--1968 & 18\,865 & 17\,036 & 15\,993 & 1045\\
%\hline
301 & Tartu Old Observatory & TT & 1947--1988 & 2275 & 2275 & 2227 & 48\\
%\hline
401 & Tautenburg Schmidt Telescope & TLS & 1960--1998 & 4101 & 20\,505 & 19\,192 & 1292\\
%\hline
501 & Zeiss Double Astrograph & VO & 1951--1999 & 544 & 544 & 532 & 13\\
\hline
\end{tabular}
\vskip 0.5cm
\caption{Digitized archives in APPLAUSE DR4. 
The abbreviations denote:
AIP  = Leibniz-Institut für Astrophysik Potsdam (AIP);
HS   = Hamburger Sternwarte;
DKRSB = Dr. Karl Remeis-Sternwarte Bamberg;
TT = Tartu Observatory, University of Tartu, Estonia;
TLS = Thüringer Landessternwarte Tautenburg;
VO = Vatican Observatory;
BSSP = Bamberg Southern Sky Patrol;
BNSP = Bamberg Northern Sky Patrol;
HSS = Hamburger Schmidt-Spiegel; 
not\_processed = most are prism plates (spectral plates), but included are scans from damaged plates which failed to process.
}
\label{dr4archives}
\end{table*}

\twocolumn
\section{Supplemental tables}

Details on the 27 archives included in the APPLAUSE data base are given in Table \ref{dr4archives}. The spatial distributions are shown in \url{https://www.plate-archive.org/cms/documentation/archives/} for each archive separately as Mollweide diagrams. Table \ref{dr4_calibsrc}
lists the number of observed epochs of \textit{Gaia} matched unique sources. \uh{More than x million} sources have more than 100 epochs of observations. In the plate archives of Hamburger Sternwarte there are substantial
numbers of photographic plates containing spectra in form of objective
prism plates or as plates with one to several single spectra and are listed in Table \ref{hamburg_stock}. The
number of these plates are given for both cases as well as the period
in which they were observed. Except
of the ESO and Calar Alto telescopes all telescopes are or were located on
the premises of Hamburger Sternwarte.
These spectroscopic plates are digitized and available in the data base but could
not been calibrated in the same way as the direct images (see Sect. \ref{sec:vo}).
 which are listed in Table \ref{hamburg_stock}.

\iffalse
\begin{table}

\centering
\begin{tabular}{ r c r  r }
\hline\hline
Bin &&& N  gaiaedr3\_id    \\
\hline
1 &-& 5&	66\,201\,983\\
6 &-&10&	25\,099\,922\\
11 &-& 20&	11\,067\,902\\
21 &-& 30&	4\,207\,168\\
31 &-& 50&	3\,919\,403\\
51 &-& 75&	2\,478\,909\\
76 &-& 100&	1\,643\,263\\
101 &-& 150&	1\,863\,840\\
151 &-& 200&	894\,082\\
201 &-& 250&	483\,292\\
251 &-& 500&	832\,894\\
501 &-& 750&	208\,227\\
751 &-& 1000&	121\,002\\
1001 &-& 1500&	36\,593\\
1501 &-& 2000&	404\\
2001&-& &	833\\
\hline
\end{tabular}
\vskip 0.5cm
\caption{Breakdown of measurement epochs for objects matched with \textit{Gaia} EDR3 source. %\_id in the APPLAUSE data base. 
Bin = number of epochs for a gedr3 source\_id;
N = count of measurements of distinct source\_id in this bin. The total number of measurements is 1.256 billion.
%\textbf{CAVEAT}: these numbers do not exclude multiple expositions on one plate.
}\label{dr4_calibsrc}
\end{table}
%\subsection*{Spectroscopic archives at Hamburger Sternwarte}
\fi

\begin{table}[h]
%\label{hh-tabn}
\centering
\begin{tabular}{c l  r  r  c  %r 
}
\hline\hline
Archive\_Id &Telescope  %&Location} 
&Prism & Single & Period \\
                     &       ID  %&      
                     & spectra & spectra &  \\
\hline
101 & HAM-LA %& HH 
& 2067 &   & 1912--56 \\
%\hline
111 & HAM-SS %& HH 
& 343  &   & 1932--54 \\
%\hline
103 & HAM-1m %& HH 
&  & 1990   & 1947--72 \\
%\hline
110 & HAM-KS %& HH 
& 225  &   & 1954--68 \\
102 &  HAM-GS %& HH  
& 2139 &    & 1955--75 \\
%\hline
104 & HS %& Calar Alto           
& 1720 &   & 1980--98 \\
%\hline
108 & ES %& La Silla             
& 738 & 398  & 1974--98 \\
%\hline
&Total  %& 
& 7232 & 2388 & 1912--98 \\
\hline
\end{tabular}
\vskip 0.5cm
\caption{Major digitized spectral archives from the Hamburg Observatory available in the APPLAUSE data base. HAM LA = Lippert-Astrograph; HAM 1m = 1m – Spiegelteleskop; HAM-SS = Original Schmidt'sches Spiegelteleskop; HAM KS =  Kleiner Schmidtspiegel II; HAM GS = Gro\ss er Schmidtspiegel (80cm) at Hamburg observatory, HS = same Schmidt telescope at Calar Alto; ES = ESO Schmidt telescope at ESO (La Silla). }
\label{hamburg_stock} 
%\label{table:hamburg_archives}
\end{table} 
%\fi

%\subfloat[first]{
 % \includegraphics[width=65mm]{test.pdf}
%}
